# Supplementary material for: Ordered Risk Minimization: Learning More from Less Data
Source: arXiv:2303.09196 source file (2023-09-18)
Supplement: Supplementary file 2 [file distortion.tex]

\section{Distortion Representation} \label{app:distortion-representation}
This section contains the proofs associated with \cref{sec:distortion-representation}.

\paragraph*{Proof of \cref{lem:identically-distributed}}  
We will need to use the vector and function characterization of random variables simultaneously throughout this proof. 
So to avoid the abuse of notation used throughout the rest 
of the paper we use capital letters when $X \colon \Omega^n \to \Re$ is 
implied and $x \in \Re^n$ for the vector representation with
\begin{equation*}
    x_i = X(\omega_i), \quad \forall i \in [n].
\end{equation*}
The random variables $X, Y \colon \Omega^n \to \Re$ are identically distributed when 
$\prob[X \in \set{X}] = \prob[Y \in \set{X}]$
for every measurable set $\set{X} \in \B$, with $\B$ the Borel sigma algebra over the reals. Using the vector representation
$\prob[X \in \set{X}] = \frac{1}{n} \sum_{i=1}^{n} \bm{1}_{\set{X}}(x_i)$.
Thus $X \deq Y$ holds iff  
\begin{equation} \label{eq:equal-distribution}
    \sum_{i=1}^{n} \bm{1}_{\set{X}}(x_i) = \sum_{i=1}^{n} \bm{1}_{\set{X}}(y_i), \quad \forall \set{X} \in \B.
\end{equation}

To show $\Leftarrow$ observe that \eqref{eq:equal-distribution} is permutation invariant. So 
$\sum_{i=1}^{n} \bm{1}_{\set{X}}(y_{\pi(i)}) = \sum_{i=1}^{n} \bm{1}_{\set{X}}(y_i)$ for all $\set{X} \in \F$. 

To show $\Rightarrow$ let $m$ denote the number of distinct elements of $x$, the values of which we define as $\{z_j\}_{j=1}^{m}$.
Then let $\set{C}_j = \{i \colon x_i = z_j\}$ for $j \in [m]$. We have 
\begin{equation*}
    \sum_{i=1}^{n} \bm{1}_{\set{X}}(x_i) = \sum_{j=1}^{m} |\set{C}_j| \bm{1}_{\set{X}}(z_j) = \sum_{i=1}^{n} \bm{1}_{\set{X}}(y_i), \quad \forall \set{X} \in \B
\end{equation*}
since $X \deq Y$ by assumption. For any $j \in [m]$ let $\set{X} = \{z_j\}$ and $\set{D}_j = \{i \colon y_i = z_j\}$. Then the above implies that $|\set{D}_j| = |\set{C}_j|$ 
for all $j \in [m]$. Take $\pi \colon [n] \to [n]$ any of the bijections such that $\pi(\set{D}_j) = \set{C}_j$. Then $y_{\pi(i)} = z_{j} = x_i$ for all $i \in \set{D}_j$ and all $j \in [m]$. 
Thus $x = \pi y$, proving the claimed result. \qed\\


% Consider $\bar{\pi}(i) = \left\{ j \colon y_j \in \{z_i\} \right\}$ and let $|\bar{\pi}(i)| = |\set{C}_i|$ for each $i \in [m]$. 
% Also, by construction $\bar{\pi}(i) \cap \bar{\pi}(j) = \emptyset$
% for each pair $i \neq j$. Hence we can define a permutation (i.e. a bijection) $\pi \colon [n] \to [n]$ by arbitrarily pairing up elements 
% between $\set{C}_i$ and $\bar{\pi}(i)$ such that $\pi^{-1}(i) \in \bar{\pi}^{-1}(i) = \set{C}_i$ for all $i \in [m]$. 
% Then taking $y = \pi x$ implies $y_{\pi^{-1}(j)} = z_i$ for $j \in \set{C}_i$ and all $i \in [m]$. Therefore 
% \begin{equation*}
%     \sum_{j=1}^{n} \bm{1}_{\set{X}}(y_j) = \sum_{j=1}^{n} \bm{1}_{\set{X}}(y_{\pi^{-1}(j)}) = \sum_{i=1}^{m} |\set{C}_i| \bm{1}_{\set{X}}(z_i).
% \end{equation*} 
% We have thus shown that \cref{eq:equal-distribution} holds. \qed

We next state the usual definition of law-invariant, coherent risk measures:
\newcommand{\cohasm}[1]{\hyperref[def:coh:#1]{\sc a\oldstylenums{#1}}}
\begin{definition}[coherent risk] \label{def:coh}
    Consider a $\rho \colon \Re^n \to \eRe$
    that is proper \footnote{
        That is $\rho(X) > -\infty$ for all $X \in \Re^n$ and the domain $\mathrm{dom}(\rho) \dfn \{X \in \Re^n \colon \rho(X) < +\infty\}$ is nonempty.
    } and lsc. Assume (for $X, Y \in \Re^n$):
    \begin{enumeratass}[leftmargin=2em]
        \item \emph{convex}: $\rho(\alpha X + (1-\alpha) Y) \leq \alpha \rho(X) + (1-\alpha) \rho(Y)$, $\forall \alpha \in [0, 1]$;\label{def:coh:1}
        \item \emph{monotone}: if $Y \geq X$, then $\rho(Y) \geq \rho(X)$;\label{def:coh:2}
        \item \emph{translation equivariance}: $\rho(X+a) = \rho(X) + a$, $\forall a \in \Re$;\label{def:coh:3}
        \item \emph{pos. homogeneity}: if $t > 0$, then $\rho(tX) = t\rho(X)$.\label{def:coh:4}
    \end{enumeratass}
    Then $\rho$ is a \emph{coherent risk measure}. Consider also
    \begin{enumeratass}[leftmargin=2em]
        \item[\textsc{A\oldstylenums{5}}.] \emph{law invariance}: if $X \deq Y$, then $\rho(Y) = \rho(X)$. \label{def:coh:5}
    \end{enumeratass}
\end{definition}
The first four assumptions were considered in \cite[\S1]{Ruszczynski2006}, while \cohasm{5} is considered in 
\cite[Def.~4.4]{Bertsimas2009b}. By \cref{lem:identically-distributed} it implies that $\rho(X) = \rho(\pi X)$ 
for all $\pi \in \Pi^n$. 

The convex conjugate $\rho^* \colon \Re^n \to \eRe$ of a risk measure is given as 
\begin{equation} \label{eq:convex-conjugate}
    \rho^*(\mu) = \sup_{X \in \Re^n} \left\{ \<\mu, X\> - \rho(X) \right\}.
\end{equation}

Its domain is affected by the assumptions in \cref{def:coh}. 
\begin{proposition} \label{prop:conjugate-duality}
    Suppose that $\rho \colon \Re^n \to \eRe$ is proper, lsc., and convex. Then, $\rho = \rho^{**}$
    with $\amb \dfn \mathrm{dom}(\rho^*)$ a non-empty and convex set. Moreover
    \begin{enumerate}[itemsep=0pt]
        \item \cohasm{2} holds iff $\mu \geq 0$ for any $\mu \in \amb$; \label{prop:conjugate-duality:2}
        \item \cohasm{3} holds iff $\sum_{i=1}^{n} \mu_i = 1$ for any $\mu \in \amb$; \label{prop:conjugate-duality:3}
        \item \cohasm{4} holds iff $\amb$ is closed and \label{prop:conjugate-duality:4}
        \begin{equation*}
            \rho(X) = \sup_{\mu \in \amb} \, \<\mu, X\>, \quad \forall X \in \Re^n
        \end{equation*}
        \item \cohasm{5} holds iff $\rho^*(\pi \mu) = \rho^*(\mu)$ for all $\pi \in \Pi^n, \mu \in \Re^n$. \label{prop:conjugate-duality:5}
    \end{enumerate}
    We assumed the underlying measure of the random variables is $\one_n/n = (1/n, \dots, 1/n)$ for (iv). 
\end{proposition}
\begin{proof}
    By \cite[Prop.~2.112]{Bonnans2000} $\rho^*$ is proper and convex. 
    Hence its domain must be non-empty and convex. 
    Now \emph{(i)}--\emph{(iii)} follows from \cite[Thm.~2.2]{Ruszczynski2006}. 

    By \cref{lem:identically-distributed}, \cohasm{5} holds iff $\rho(\pi X) = X$ for all $\pi \in \Pi^n$. 
    We first show that \cohasm{5} implies $\rho^*(\pi \mu) = \rho^*(\mu)$ for all $\pi \in \Pi^n$.
    First note that 
    \begin{align*}
        &\sup_{X} \left\{ \<\mu, X\> - \rho(X) \right\} = \sup_{X} \left\{ \<\mu, \pi(X)\> - \rho(\pi(X)) \right\} \\
        &\qquad = \sup_{X} \left\{ \<\pi^{-1}(\mu), X\> - \rho(X) \right\}
    \end{align*}
    Since $\{\pi^{-1} \colon \pi \in \Pi^n\} = \Pi^n$ we have shown $\rho^*(\pi \mu) = \rho^*(\mu)$ for all $\mu \in \Re^n$
    and all $\pi \in \Pi^n$. For the reverse implication we can apply the same reasoning and using that $\rho = \rho^{**}$. 
    Note that this result specializes \cite[Prop.~2]{Shapiro2013}.
\end{proof}

% Note that \cref{def:ambiguity} is a direct consequence of \cref{prop:conjugate-duality}.
% Hence the definition is consistent with the usual definition of law-invariant coherent risk measures in \cref{def:coh}. 

% As discussed in \cref{sec:distortion-representation} we will derive an analogous representation to 
% the ambiguity representation in \cref{def:ambiguity} using the ordered convex conjugate:
% \begin{equation} 
%     \rho^{\diamond}(\mu) \dfn \sup_{X \in \M^n} \left\{ \<\mu, X\> - \rho(X) \right\}. \tag{\ref{eq:ordered-conjugate}}
% \end{equation}
To find the equivalent of \cref{prop:conjugate-duality} for the ordered conjugate $\rho^\diamond$, we
begin by relating $\rho^\diamond$ to $\rho^*$ in terms of an infimal convolution.
Then we relate their domains.
\begin{lemma} \label{lem:infimal-convolution}
    Given some proper, convex, lsc. and law-invariant risk measure $\rho \colon \Re^n \to \eRe$. Then 
    \begin{equation*}
        \rho^{\diamond} = (\rho + \indi_{\M^n})^* = \rho^* \episum \indi_{(\M^n)^\circ}.
    \end{equation*}
\end{lemma}
\begin{proof}
    The first equality holds by definition of the conjugate and the indicator. 
    Plugging in the associated definitions and changing signs makes the second equality equivalent to
    \begin{align*}
        \inf_{x} \, \rho(x) + (\indi_{\M^n}(x) - \<x, y\>) = - \inf_u \rho^*(u) + \indi^*_{\Re^n_{\uparrow}}(y-u).
    \end{align*}
    Letting $f(x) = \rho(x)$ and $g(x) = \indi_{\M^n}(x) - \<x, y\>$. Note that $f^{*} = \rho^*$ and $g^*(u) = \indi^*_{\M^n}(y+u)$. 
    Thus we require
    \begin{align*}
        \inf_x \, f(x) + g(x) = - \inf_u f^{*}(u) + g^{*}(-u),
    \end{align*}
    which by \cite[Fact.~15.25]{Bauschke2011}, since $g$ is polyhedral, requires $\dom g \cap \ri \dom f \neq \emptyset$. 
    
    By properness, $\dom \rho \neq \emptyset$, which by convexity of $\rho$ and \cite[Fact.~6.14(i)]{Bauschke2011} implies $\ri \dom \rho \neq \emptyset$.
    Moreover, by permutation invariance $x \in \dom \rho$ implies $\pi x \in \dom\rho$ for all $\pi \in \Pi^n$ since $\rho(\pi(x)) = \rho(x) < \infty$. 
    Thus $\pi \dom \rho = \dom \rho$. Moreover, by \cite[Prop.~2.44]{Rockafellar1998} and linearity of permutations we have $\ri (\dom \rho) = \ri (\pi \dom \rho) = \pi \ri (\dom \rho)$. 
    Thus $\dom g \cap \ri \dom f = \Re^n_{\uparrow} \cap \ri (\dom\rho) \neq \emptyset$. 

    Finally note that $\indi_{\M^n}^* = \indi_{(\M^n)^\circ}$ by \cite[Ex.~11.4]{Rockafellar1998}. 
\end{proof}

\begin{proposition} \label{prop:fundamental-equivalence-lemma}
    Let $\rho \colon \Re^n \to \eRe$ be lsc., convex and law-invariant risk measure. 
    Then
    \begin{align*}
        \mathrm{dom}\left( \rho^{\diamond} \right) &= \mathrm{dom}\left( \rho^* \right) + (\M^n)^\circ \\
        \mathrm{dom}\left( \rho^* \right) &= \bigcap_{\pi \in \Pi^n} \pi\left( \mathrm{dom}\left( \rho^{\diamond} \right) \right).
    \end{align*}
\end{proposition}
\begin{proof}
    The first result follows from \cref{lem:infimal-convolution} and \cite[Ex.~1.28]{Rockafellar1998}. %
    The second result follows from \cref{cor:cone-shift-invariance}. 
\end{proof}

The equivalence derived through \cref{prop:fundamental-equivalence-lemma} enables us to 
re-derive many of the statements in \cref{prop:conjugate-duality} for $\rho^\diamond$. 

\begin{proposition} \label{prop:ordered-conjugate-duality}
    Suppose that $\rho \colon \Re^n \to \eRe$ is lsc., law-invariant and convex. Then
    $\distort \dfn \mathrm{dom}(\rho^\diamond)$ is a convex set such that $\distort \cap \M^n \neq \emptyset$. 
    Moreover
    \begin{enumerate}[itemsep=0pt]
        \item If $\mu \in \distort$ then $\mu + (\M^n)^\circ \subseteq \distort$;
        \item \cohasm{2} holds iff any $\mu$ s.t. $\pi(\mu) \in \distort$ for all permutations $\pi \in \Pi^n$
        is nonnegative. 
        \item \cohasm{3} holds iff $\sum_{i=1}^{n} \mu_i = 1$ for any $\mu \in \distort$; 
        \item \cohasm{4} holds iff $\distort$ is closed and
        \begin{equation*} 
            \rho(X) = \sup_{\mu \in \distort} \, \<\mu, X_{\uparrow}\>, \quad \forall X \in \Re^n
        \end{equation*}
    \end{enumerate}
\end{proposition}
\begin{proof}
    By \cref{prop:conjugate-duality} we have convexity of $\dom\rho^*$. This implies convexity of $\rho^\diamond$ 
    (Minkowski sum of convex sets). Next assume $x \in \dom \rho^*$ then, by \cref{prop:fundamental-equivalence-lemma}, 
    $\pi(x) \in \distort$ for all $\pi \in \Pi^n$. Thus $x_{\uparrow} \in \distort$. 
    So $\dom \rho^* \neq \emptyset$, which holds by \cref{prop:conjugate-duality}, implies $\distort \cap \M^n \neq \emptyset$.
    % Similarly, assume there is some $\mu_{\uparrow} \in \distort \cap \M^n \neq \emptyset$. 
    % By \cref{prop:permuto-hull} we have $\hull (\Pi^n \mu) \in \mu_{\uparrow} + (\M^n)^\circ$.
    % Thus $\pi(\hull (\Pi^n \mu)) \in \distort$ for all $\pi$ or equivalently $\hull (\Pi^n \mu) \subseteq \cap_{\pi} \pi(\distort)$. 
    % Note that $\dom \rho^* = \cap_{\pi} \pi(\distort)$ by \cref{prop:permuto-hull}. So $\dom\rho^* \neq \emptyset$.
    
    \emph{(i)} holds by \cref{prop:fundamental-equivalence-lemma}. To show \emph{(ii)} we use \cref{prop:fundamental-equivalence-lemma}
    and specifically $\dom \rho^* = \cap_{\pi} \pi(\distort)$. So $x \in \dom \rho^*$ iff $\pi(x) \in \distort$ for all $\pi \in \Pi^n$.
    Note that \cohasm{2} holds iff $x \geq 0$ for all $x \in \dom \rho^*$. So \cohasm{2} holds iff every $x$ such that $\pi(x) \in \distort$ for all $\pi \in \Pi^n$
    is nonnegative, proving \emph{(ii)}.

    Let $\bar{\rho} = \rho + \iota_{\Re^n}$ as in \cref{lem:infimal-convolution}.
    Then $\distort = \mathrm{dom}(\bar{\rho}^*)$. 
    By permutation invariance $\bar{\rho}(X_{\uparrow}) = \rho(X_{\uparrow}) = \rho(X)$ for all $X \in \Re^n$. 
    We can then prove \emph{(iii)} by noting that $(X + a)_{\uparrow} = X_{\uparrow} + a$. 
    Hence \cohasm{3} holds for $\bar{\rho}$
    iff it holds for $\rho(X) = \bar{\rho}(X_{\uparrow})$. Thus we can apply \cref{prop:conjugate-duality:3} 
    to $\bar{\rho}$ in order to link \cohasm{3} with $\mathrm{dom}(\rho^{\diamond}) = \mathrm{dom}(\bar{\rho}^{*})$. 
    For \emph{(iv)} we use a similar argument noting that $(\alpha X)_{\uparrow} = \alpha X_{\uparrow}$ for all $X \in \Re^n$
    and all $\alpha \geq 0$ and apply \cref{prop:conjugate-duality:4}. The only property of $\rho$ 
    that does not transfer to $\bar{\rho}$ is monotonicity. So \emph{(ii)} is more complex. 
\end{proof}

We can now prove the main theorem of \cref{sec:distortion-representation}.
\paragraph*{Proof of \cref{thm:distortion-representation}} 
We need to show that \cref{prop:ordered-conjugate-duality} implies the properties of $\distort$
as stated in the theorem. \cref{prop:ordered-conjugate-duality} directly implies the following properties:
convexity, closedness, \emph{(ii)}, \emph{(iii)} and \emph{(iv)} as well as \cref{eq:distortion-representation}. 
The one remaining property is \emph{(i)}. Note that, for any $\mu \in \dom\rho^*$ we have 
$\hull(\Pi^n \mu) \subseteq \dom \rho^*$ by permutation invariance (so $\mu_{\uparrow} \in \dom\rho^*$).
Then \cref{prop:fundamental-equivalence-lemma} and \cref{prop:permuto-hull} imply $\hull(\Pi^n \mu) \subseteq \dom \rho^\diamond$. 
Take $E \in \Re^{n \times n}$ a matrix of all ones. 
Then $E\mu/n \in \hull(\Pi^n \mu) $. Since $\sum_{i=1}^{n} \mu_i = 1$ by \emph{(iii)} we have 
$E\mu/n = \one_n /n$. So if $\one_n /n \notin \dom \rho^*$ then $\dom \rho^*$ 
is empty by contradiction. Thus $\distort$ contains $\one_n/n$ since otherwise $\dom\rho^* = \emptyset$.
Finally, \cref{eq:distort-ambiguity-relation} rephrases \cref{prop:fundamental-equivalence-lemma}. \qed{}
