# Supplementary material for: Ordered Risk Minimization: Learning More from Less Data
Source: arXiv:2303.09196 source file (2023-09-18)
Supplement: Supplementary file 3 [file monotone.tex]

\section{Monotone Cone}
Let $\Re^n_{\uparrow} \dfn \{x \in \Re^n \colon x_1 \leq x_2 \leq \dots \leq x_n\}$ 
denote the monotone cone. This cone and its dual have a history in isotonic regression \cite{Barlow1972}
and majorization \cite{Steerneman1990}. 

% We begin by deriving the polar of $\Re^n_{\uparrow}$. The following property will be useful for this.
% \begin{lemma} \label{lem:inner-product}
%     Let $x, y \in \Re^n$ and $x_{0} = 0$. Then 
%     \begin{equation*}
%         \ssum_{i=1}^{n} x_i y_i = \ssum_{i=1}^{n} (x_{i} - x_{i-1}) \left( \ssum_{j=i}^{n} y_j \right).
%     \end{equation*}
% \end{lemma}
% \begin{proof}
%     For some $k \in [n]$, $x_k$ enters in the sum on the right-hand side for $i = k$ and $i=k+1$.
%     The full term is thus
%     \begin{align*}
%         x_k \left(\ssum_{j=k}^{n} y_j\right) - x_k \left(\ssum_{j=k+1}^{n} y_j\right) = x_k y_k.
%     \end{align*}
%     Using this argument for each $k$ completes the proof. 
% \end{proof}

We derive the polar of $\M^n$.
\begin{lemma} \label{prop:dual-monotone-cone}
    Let $\M^n$ be the monotone cone.
    Then 
    \begin{align*}
        (\M^n)^\circ = \left\{ x \in \Re^n \colon \sum_{i=1}^k x_i \geq 0, \forall k \in [n-1], \sum_{i=1}^n x_i = 0 \right\}. 
    \end{align*}
\end{lemma}
\begin{proof}
    The monotone cone is polyhedral with $\M^n = \{x \colon Mx \leq 0\}$ for 
    $M \in \Re^{n-1 \times n}$ with $Mx = (x_1 - x_2, x_2 - x_3, \dots, x_{n-1} - x_n)$. 
    The definition of the polar cone is thus 
    \begin{align*}
        (\M^n)^\circ &= \left\{ y \in \Re^n \colon \<x, y\> \leq 0, \forall x \text{ s.t. } M x \leq 0 \right\}.
    \end{align*}
    By Farkas' lemma \cite[p.~263]{Boyd2004} we have either $Mx \leq 0$ and $\<x, y\> > 0$ or $\trans{M} \lambda = y$ and $\lambda \geq 0$. 
    So
    \begin{align*}
        (\M^n)^\circ = \left\{ y \in \Re^n \colon y = \trans{M} \lambda, \lambda \geq 0 \right\}.
    \end{align*}
    Note that $\<\lambda, Mx\> = \sum_{i=1}^{n-1} \lambda_i (x_i - x_{i+1}) = \sum_{j=1}^{n} x_j (\lambda_{j} - \lambda_{j-1}) = \<\trans{M} \lambda, x\>$,
    where $\lambda_0 = \lambda_{n} = 0$. Thus $y \in (\M^n)^\circ$ iff $y = \trans{M} \lambda$ for $\lambda \geq 0$. Here $y = \trans{M} \lambda$ holds iff 
    \begin{align*}
        y_j &= \lambda_j - \lambda_{j-1}, &&\forall j \in [n].  \\
        \Leftrightarrow \quad \ssum_{j=1}^k y_j &= \ssum_{j=1}^k \lambda_j - \lambda_{j-1} = \lambda_k, &&\forall k \in [n]. 
    \end{align*}
    Since $\lambda \geq 0$ we have $\sum_{j=1}^k y_j = \lambda_k \geq 0$ for $k \in [n-1]$ and $\sum_{j=1}^{n} y_j = \lambda_n = 0$. 
    % We can rewrite the inner product using \cref{lem:inner-product} as
    % \begin{equation*}
    %     \ssum_{i=1}^{n} (y_{(i)} - y_{(i-1)}) ( \ssum_{j=i}^{n} x_j ) \leq 0, \quad \forall y \in \Re^n.
    % \end{equation*}
    % First note that $y_{(1)} - y_{(0)} = y_{(1)}$ has arbitrary sign.
    % Since $y_{(1)} - y_{(0)} = y_{(1)}$ has arbitrary sign, we have $\sum_{i=1}^{n} x_i = 0$.  
    % Note that $y_{(i)} \geq y_{(i-1)}$ for all $i \in [2, n]$. Therefore, $\forall k \in [n-1]$,
    % \begin{align*}
    %     \ssum_{i=k+1}^n x_i \leq 0 \, &\Leftrightarrow \, \ssum_{i=1}^{n} x_i - \ssum_{i=k+1}^n x_i \geq 0 \\
    %     &\Leftrightarrow \, \ssum_{i=1}^{k} x_i \geq 0,
    % \end{align*}
    % thereby proving the required result.
\end{proof}

% The cone is deeply linked to the permutation group $\Pi^n$ of bijections $\pi \colon [n] \to [n]$. 
% Consider \cite[Eq.~2.2]{Steerneman1990}
% \newcommand{\match}{\mmathcal{m}}
% \begin{definition}
%     Consider the \emph{matching function}
%     \begin{equation*}
%         \match(u, x) = \sup_{\pi \in \Pi^n} \, \<u, \pi x\>, \quad \forall x,u \in \Re^n.
%     \end{equation*}
% \end{definition}

% The matching function was introduced to study group induced cone orderings (e.g. majorization) \cite{Steerneman1990}.
% The ordering induced by the permutation group is majorization \cite{Marshall2011}:
% \begin{definition}
%     For $x, y \in \Re^n$, then $x \slt y$ iff $x \in \hull (\Pi^n y)$. 
% \end{definition}

% We first link matching with majorization \cite[\S2]{Steerneman1990}
% \begin{proposition}
%     For $x, y \in \Re^n$, then $x \slt y$ iff
%     \begin{equation*}
%         \match(u, x) \leq \match(u, y) \quad \text{for all } u \in \Re^n.
%     \end{equation*} 
%     % which holds iff $x_{\uparrow} - y_{\uparrow} \in (\M^n)^\circ$.
% \end{proposition}

% Meanwhile matching relates to $\M^n$ as follows 
% \begin{proposition} \label{prop:fundamental-region}
%     For each $x, y \in \M^n$: 
%     \begin{enumerate}[(i)]
%         \item $\Pi^n x \cap \M^n \neq \emptyset$; \, (ii) $\match(x, y) = \<x, y\>$
%     \end{enumerate}
% \end{proposition}
% \begin{proof}
%     \emph{(ii)} follows by \cite[Prop.~6.A.3]{Marshall2011} and \emph{(i)} follows by noting 
%     that $\exists \pi \in \Pi^n$ s.t. $\pi(x) = x_{\uparrow}$.
% \end{proof}
% The above facts identify $\M^n$ as the closure of a \emph{fundamental region} \cite[Thm.~3.1]{Steerneman1990}
% and $x \slt y$ as a \emph{group-induced cone ordering} \cite[Def.~2.1]{Steerneman1990}.
% This has several consequences. Most importantly it implies the following \cite[\S2]{Steerneman1990}:
% \begin{proposition} \label{prop:group-induced-cone-order}
%     Consider $x, y \in \Re^n$. Then 
%     \begin{equation*}
%         x \slt y \quad \text{iff} \quad x_{\uparrow} - y_{\uparrow} \in (\M^n)^\circ.
%     \end{equation*}
% \end{proposition}

We relate $(\M^n)^\circ$ to majorization. 
\begin{lemma} \label{prop:group-induced-cone-order}
    Consider $x, y \in \Re^n$. Then
    \begin{equation*}
        x_{\uparrow} \in y_{\uparrow} + (\M^n)^\circ \quad \text{iff} \quad x \slt y,
    \end{equation*}
    where $x \slt y$ denotes that $x$ is majorized by $y$. 
\end{lemma}
\begin{proof}
    The definition of majorization \cite[Def.~1.A.1]{Marshall2011} is:
    \begin{align*}
        x \slt y \, \Leftrightarrow \, \sum_{i=1}^{n} x_{(i)} \geq \sum_{i=1}^{n} y_{(i)} \text{ and } \sum_{i=1}^{n} x_i = \sum_{i=1}^{n} y_i.
    \end{align*}
    This is clearly equivalent to \cref{prop:dual-monotone-cone} applied to $x_{\uparrow} - y_{\uparrow}$. 
\end{proof}

% The characterization in terms of a group-induced cone ordering also implies the following 
% characterization of the convex hulls of the orbit under $\Pi^n$:
Majorization is related to the convex hull of the orbit under $\Pi^n$. Specifically \cite[Cor.~2.B.3]{Marshall2011}:
\begin{equation} \label{eq:permuto-hull-eq}
    x \slt y \quad \Leftrightarrow \quad x \in \hull(\Pi^n y). 
\end{equation}

This has the following useful consequence.
\begin{lemma} \label{prop:permuto-hull}
    Consider $y \in \Re^n$. Then 
    \begin{equation*}
        \hull (\Pi^n y) = \bigcap_{\pi \in \Pi^n} \pi(y_{\uparrow} + (\M^n)^\circ).
    \end{equation*}
    % \begin{enumerate}[(i)]
    %     \item \label{prop:permuto-hull:a} $\hull (\Pi^n y) \subseteq y_{\uparrow} + (\M^n)^\circ$; 
    %     \item \label{prop:permuto-hull:b} 
    %     % \item $\hull (\Pi^n y) = \cup_{\pi \in \Pi^n} \pi(\M^n \cap (y + (\M^n)^\circ))$.
    % \end{enumerate}
\end{lemma}
\begin{proof}
    The result is a specialization of \cite[Lem.~4.2]{Steerneman1990}. Take $x \in \hull (\Pi^n y)$.
    Then $x \slt y$ by \cref{eq:permuto-hull-eq} and $x_{\uparrow} - y_{\uparrow} \in (\M^n)^\circ$ by \cref{prop:group-induced-cone-order}.
    Using the definition of the polar cone this gives:
    \begin{align*}
        &\<x_{\uparrow} - y_{\uparrow}, u_{\uparrow}\> \leq 0, &&\forall u_{\uparrow} \in \M^n \\
        \Leftrightarrow \quad &\<x_{\uparrow}, u_{\uparrow}\> \leq \<y_{\uparrow}, u_{\uparrow}\>, &&\forall u_{\uparrow} \in \M^n \\
        \Rightarrow \quad &\<x, u_{\uparrow}\> \leq \<y_{\uparrow}, u_{\uparrow}\>, &&\forall u_{\uparrow} \in \M^n, \\
        \Leftrightarrow \quad &x - y_{\uparrow} \in (\M^n)^\circ,
    \end{align*}
    where we used $\<x, u_{\uparrow}\> \leq \<x_{\uparrow}, u_{\uparrow}\>$ \cite[Prop.~6.A.3]{Marshall2011} for the third implication
    and the definition of the polar cone again for the fourth. Thus we have shown that $x \in y_{\uparrow} + (\M^n)^\circ$.
    As we could have taken any $x \in \hull(\Pi^n y)$ we thus showed $\hull (\Pi^n y) \subseteq y_{\uparrow} + (\M^n)^\circ$.
    We can take permutations of both sides without affecting the result (since permutations are invertible). Moreover $\pi \hull(\Pi^n y) = \hull(\Pi^n y)$.
    Thus $\hull (\Pi^n y) \subseteq \pi(y_{\uparrow} + (\M^n)^\circ)$ for all $\pi \in \Pi^n$ and $\hull (\Pi^n y) \subseteq \cap_{\pi} \pi(y_{\uparrow} + (\M^n)^\circ)$. 

    For the converse let $x \in \cap_{\pi \in \Pi^n} \pi(y_{\uparrow} + (\M^n)^\circ)$. So $x_{\uparrow} \in y_{\uparrow} + (\M^n)^\circ$. 
    By \cref{prop:group-induced-cone-order} we have $x \slt y$. Applying \cref{eq:permuto-hull-eq} then implies $x \in \hull(\Pi^n y)$.
    Therefore $\cap_{\pi \in \Pi^n} \pi(y_{\uparrow} + (\M^n)^\circ) \subseteq \hull(\Pi^n y) $, completing the proof.
\end{proof}

We can generalize the above to apply to convex, permutation invariant sets. 
\begin{proposition} \label{cor:cone-shift-invariance}
    Consider some convex permutation invariant $\set{A} \subseteq \Re^n$ (i.e. $x \in \set{A}$ implies $\pi x \in \set{A}$ for all $\pi \in \Pi^n$).
    Then 
    \begin{equation*}
        \set{A} = \bigcap_{\pi \in \Pi^n} \pi(\set{A} + (\M^n)^{\circ}).
    \end{equation*}
\end{proposition}
\begin{proof}
    Let $x \in \set{A}$. Since the identity map is also in $\Pi^n$, \cref{prop:permuto-hull} implies $\hull(\Pi^n x) \subseteq x_{\uparrow} + (\Re^n_{\uparrow})^\circ$.
    Therefore we have $\pi(x) \in x_{\uparrow} + (\M^n)^\circ$ for all $\pi \in \Pi^n$. 
    Noting that $x_{\uparrow} \in \set{A}$ by permutation invariance gives $\pi(x) \in \set{A} + (\Re^n_{\uparrow})^\circ$ for all $\pi \in \Pi^n$. 
    For every $\pi \in \Pi^n$, also $\pi^{-1} \in \Pi^n$. We can apply this inverse to both sides of the inclusion.
    Thus $x \in \cap_{\pi} \pi(\set{A} + (\M^n)^\circ)$ and $\set{A} \subseteq \cap_{\pi} \pi(\set{A} + (\M^n)^\circ)$.

    For the converse let $x \in \cap_{\pi} \pi(\set{A} + (\M^n)^\circ)$. Then, again since $\pi^{-1} \in \Pi^n$, $\pi(x) \in \set{A} + (\M^n)^\circ$ for all $\pi \in \Pi^n$.
    Specifically $x_{\uparrow} \in \set{A} + (\M^n)^\circ$, which implies $\exists y \in \set{A}$ such that $x_{\uparrow} \in y + (\M^n)^\circ$. 
    Note that $y \in y_{\uparrow} + (\M^n)^\circ$ by \cref{prop:permuto-hull}. That is $\exists s \in (\M^n)^\circ$ such that $y = y_{\uparrow} + s$
    and $x_{\uparrow} \in y + s + (\M^n)^\circ$. Since $(\M^n)^\circ$ is a convex cone, $s + s' \in (\M^n)^\circ$ for $s, s' \in (\M^n)^\circ$.
    Thus $x_{\uparrow} \in y_{\uparrow} + (\M^n)^\circ$, which by \cref{prop:group-induced-cone-order} implies $x \slt y$ or $x \in \hull(\Pi^n y)$ \cref{eq:permuto-hull-eq}. 
    From $y \in \set{A}$ and permutation invariance $\Pi^n y \subseteq \set{A}$. Moreover, by convexity, $\hull(\Pi^n y) \subseteq \set{A}$. Thus $x \in \set{A}$ 
    and $\cap_{\pi} \pi(\set{A} + (\M^n)^\circ) \subseteq \set{A}$. 
\end{proof}

We finish with a characterization of the convex hull of the permutations of some vector as a polyhedral set.
\begin{proposition} \label{lem:simple-distortion-characterization}
    Consider a vector $x \in \Re^n$ with $d$ distinct elements, which we store in $\bar{x} \in \Re^d$. Let $c \in \N^d$ denote 
    the number of copies of each component of $\bar{x}$ in $x$. Then 
    \begin{align*}
        \hull\left( \Pi^n x \right) = \{ S\bar{x} \colon S\one_d = \one_n, \trans{\one}_n S = \trans{c}, S \geq 0\}.
    \end{align*}
\end{proposition}
\begin{proof}
    Since the doubly stochastic matrices are the convex hull of the permutation matrices \cite[2.A.2]{Marshall2011}, the convex hull of all permutations of $x$ is
    \begin{equation*}
        \hull\left( \Pi^n x \right) = \left\{ H x \colon H \one_n = \one_n, \trans{\one}_n H = \one_n, H \geq 0 \right\}.
    \end{equation*}
    Consider
    \begin{equation*}
        \trans{C} \dfn \smallmat{
            1 & \dots & 1 \\ &&& \ddots \\ &&&& 1 & \dots & 1
         } \in \Re^{d \times n},
    \end{equation*}
    where row $i$ contains $c_i$ repetitions of $1$ for each $i \in [d]$ such that $x = C \bar{x}$. The pseudo-inverse $C^{\dagger}$ is given as 
    \begin{equation*}
        C^{\dagger} \dfn \smallmat{
            1/c_1 & \dots & 1/c_1 \\ &&& \ddots \\ &&&& 1/c_d & \dots & 1/c_d
        } \in \Re^{d \times n}.
    \end{equation*}
    So $\bar{x} = C^{\dagger} x$ and $C^{\dagger} C = I_d$. 

    Take $H$ doubly stochastic. Then $v = H C C^{\dagger} x = HC \bar{x} \in \hull\left( \Pi^n x \right)$ and $S = HC$ satisfies the conditions above. 
    Specifically  $H \trans{C} \one_d = H \one_n = \one_n$ and $\trans{\one_n} H \trans{C} = \trans{\one_n} \trans{C} = \trans{\one_d}$ and $H \trans{C} \geq 0$.
    Let $\set{R}$ denote the right-most set in the proposition. We have shown $v \in \set{R}$ or $\hull\left( \Pi^n x \right) \subseteq \set{R}$. 
    For the reverse implication take some $v \in \set{R}$. So $v = S y = S C^{\dagger} C y = S C^{\dagger} x$. It is easy to verify that $S C^{\dagger}$ is doubly stochastic.
    Thus $v \in \hull\left( \Pi^n x \right)$. 
\end{proof}


% \section{Monotone Cone}

% Consider the monotone cone. We first derive its dual. 
% \begin{lemma} \label{lem:dual-monotone-cone}
%     Let $\M^n$ be the monotone cone.
%     Then 
%     \begin{align*}
%         (\M^n)^\circ &\dfn (\M^n)^\circ \\
%         &= \left\{ x \in \Re^n \colon \sum_{i=k}^n x_i \leq 0, \forall k \in [2, n], \sum_{i=1}^n x_i = 0 \right\}. 
%     \end{align*}
% \end{lemma}
% \begin{proof}
%     Plugging in the definition of the dual cone gives 
%     \begin{align*}
%         (\M^n)^\circ &= \left\{ y \in \Re^n \colon \<x, y\> \leq 0, \forall x \in \M^n \right\}.
%     \end{align*}
%     We can replace the inner product using \cref{cor:inner-product} with 
%     \begin{equation*}
%         \ssum_{i=1}^{n} (x_{(i)} - x_{(i-1)}) ( \ssum_{j=i}^{n} y_j ) \leq 0, \quad \forall x \in \Re^n
%     \end{equation*}
%     Note that $x_{(i)} \geq x_{(i-1)}$ for all $i \in [2, n]$, which gives the first set of constraints. 
%     The final constraint follows by noting that $x_{(1)} - x_{(0)} = x_{(1)}$ has arbitrary sign.  
% \end{proof}

% We do the same for the nonnegative monotone cone.
% \begin{lemma} \label{lem:dual-nn-monotone-cone}
%     Let $\pM^n$ be the nonnegative monotone cone.
%     Then 
%     \begin{align*}
%         (\M^n)^\circ_+ &\dfn (\pM^n)^* = \left\{ x \in \Re^n \colon \sum_{i=k}^n x_i \geq 0, \forall k \in [n] \right\}. 
%     \end{align*}
% \end{lemma}
% \begin{proof}
%     The proof is analogous to that of \cref{lem:dual-nn-monotone-cone}. Except for the final step where we known $x_{(1)} \geq 0$.
% \end{proof}

% We consider properties of the \emph{cumulative cone}. We first derive a generator characterization.
% \begin{lemma} \label{lem:cumulative-cone}
%     Let $(\M^n)^\circ$ be as given in \cref{lem:dual-monotone-cone}. Then
%     \[(\M^n)^\circ = \{(\tau_2-\tau_1, \tau_3 - \tau_2, \dots, -\tau_{n}) \colon \tau \in \Re^{n}_+, \tau_1 = 0\}.\]
% \end{lemma}
% \begin{proof}
%     Take some $x \in (\M^n)^\circ$ and let $\tau_{k} = -\sum_{i=k}^{n} x_i$ for $k \in [n]$.
%     Since $x \in (\M^n)^\circ$ we have $\tau \in \Re^{n}_+$ and $\tau_1 = 0$. Moreover
%     \begin{align*}
%         &(\tau_2-\tau_1, \dots, -\tau_{n}) \\
%         &= (\ssum_{i=1}^{n}x_i - \ssum_{i=2}^{n}x_i, \dots, \ssum_{i=n}^{n}x_i) \\
%         &= (x_1, \dots, x_n).
%     \end{align*}
%     To show the other inclusion let $\tau \in \Re^{n}_+$ and $\tau_1 = 0$ and $(x_1, \dots, x_n) = (\tau_2-\tau_1, \dots, -\tau_{n})$. 
%     Then $\sum_{i=k}^{n} x_i = -\tau_k \leq 0$ for $k \in [2, n]$ and $\sum_{i=1}^n x_i = \tau_1 = 0$. 
% \end{proof}

% We prove some properties of $(\M^n)^\circ$ related to permutations.
% \begin{lemma} \label{lem:permutation-hull-contained}
%     Let $(\M^n)^\circ$ be as in \cref{lem:dual-monotone-cone}. Then, $\forall x \in \Re^n$,
%     \begin{equation*}
%         \hull\left( \{\pi(x) \colon \pi \in \Pi^n\} \right) \subset x_{\uparrow} + (\M^n)^\circ. 
%     \end{equation*}
% \end{lemma}
% \begin{proof}
%     We begin by showing that for every $x$ we have $x \in x_{\uparrow} + (\M^n)^\circ$, which holds iff 
%         $x - x_{\uparrow} \in (\M^n)^\circ$
%     Let $g^{(k)} = (0, \dots, 0, 1, \dots, 1) \in \Re^n$ the $k$'th row of $G$ as in \cref{lem:upper-triangular}. 
%     Since clearly $\sum_{i=1}^{n} x_{i} - x_{(i)} = 0$ we should only show, for all $k \in [2, n]$, 
%     \begin{align*}
%         &\langle g^{(k)}, x - x_{\uparrow} \rangle = \sum_{i=1}^{n} g^{(k)}_i (x_{i} - x_{(i)}) \leq 0,
%     \end{align*}
%     which by construction implies $x - x_{\uparrow} \in (\M^n)^\circ$.
%     The above inequality holds iff 
%     \begin{align*}
%         &\Leftrightarrow \quad \sum_{i=1}^{n} g^{(k)}_{(i)} x_{i} \leq \sum_{i=1}^{n} g^{(k)}_{(i)} x_{(i)} \\
%         &\Leftrightarrow \quad \sum_{i=1}^{n} g^{(k)}_{[i]} x_{n-i+1} \leq \sum_{i=1}^{n} g^{(k)}_{[i]} x_{[i]}
%     \end{align*}
%     where we used the fact that $g^{(k)}_{\uparrow} = g^{(k)}$
%     and $x_{[i]} = x_{(n - i + 1)}$. The final inequality follows from \cite[Prop.~6.A.3]{Marshall2011}.

%     Thus we have shown that $\pi(x_{\uparrow}) \in x_{\uparrow} + (\M^n)^\circ$ for all $\pi \in \Pi^n$. 
%     Adding $x_{\uparrow}$ does not affect convexity of $(\M^n)^\circ$.
%     So since $\pi(x) \in x_{\uparrow} + (\M^n)^\circ$ for all $\pi \in \Pi^n$ with a convex right-hand side
%     we conclude $\hull\left( \{\pi(x) \colon \pi \in \Pi^n\} \right) \subset x_{\uparrow} + (\M^n)^\circ$.
% \end{proof}

% \begin{lemma} \label{lem:opposite-hull-contained}
%     For any $x \in \Re^n$ such that $x \neq x_{\uparrow}$
%     \begin{equation*}
%         \exists \pi \in \Pi^n\colon \pi(x) \notin x + (\M^n)^\circ.
%     \end{equation*}
% \end{lemma}
% \begin{proof}
%     The proof is similar to that of \cite[Thm.~368]{Hardy1952}. We have $\pi(x) \notin x + (\M^n)^\circ$ iff 
%     \begin{equation*}
%         \exists k \in [2, n]\colon \<g^{(k)}, \pi(x)\> > \<g^{(k)}, x\>,
%     \end{equation*}
%     with $g^{(k)} = (0, \dots, 0, 1, \dots, 1) \in \Re^n$ the $k$'th row of $G$ as in \cref{lem:upper-triangular}.
%     Take $i$ such that $x_{i} > x_{i+1}$, which exist by $x \neq x_{\uparrow}$. Take $k$ such that $g^{(k)}_{i} = 0$
%     and $g^{(k)}_{i+1} = 1$ (i.e. $k = i + 1$). Let $\pi(i) = i+1$, $\pi(i+1) = i$ and $\pi(j) = j$ for all $j \in [n] \setminus \{i, i+1\}$. 
%     Then
%     \begin{align*}
%         \<g^{(k)}, \pi(x)\> &= \ssum_{j=i+2}^n x_j + x_{i} \\ &> \ssum_{j=i+2}^n x_j + x_{i+1} = \<g^{(k)}, x\>,
%     \end{align*}
%     which completes the proof.
% \end{proof}

% We relate $(\M^n)^\circ$ to majorization. 
% \begin{lemma} \label{lem:majorization}
%     Consider $x, y \in \Re^n$ and $(\M^n)^\circ \dfn (\M^n)^\circ$. Then
%     \begin{equation*}
%         x_{\uparrow} \in y_{\uparrow} + (\M^n)^\circ \quad \text{iff} \quad x \slt y,
%     \end{equation*}
%     where $x \slt y$ denotes that $x$ is majorized by $y$. 
% \end{lemma}
% \begin{proof}
%     Note that $x_{\uparrow} - y_{\uparrow} \in (\M^n)^\circ$ holds iff $\sum_{i=1}^{n} x_i - y_i = 0$ and $\forall k \in [2, n]$,
%     \begin{align*}
%         &&\ssum_{i=k}^{n} x_{(i)} - y_{(i)} &\leq 0 \\
%         &\Leftrightarrow&-\ssum_{i=k}^{n} x_{(i)} &\geq -\ssum_{i=k}^{n} y_{(i)} \\
%         &\Leftrightarrow&\ssum_{i=1}^{n} x_{i} - \ssum_{i=k}^{n} x_{(i)} &\geq \ssum_{i=1}^{n} y_{i} - \ssum_{i=k}^{n} y_{(i)} \\
%         &\Leftrightarrow&\ssum_{i=1}^{k-1} x_{(i)} &\geq \ssum_{i=1}^{k-1} y_{(i)}. 
%     \end{align*}
%     The last inequality and $\sum_{i=1}^{n} x_i - y_i = 0$ defines $x \slt y$ \cite[Def.~1.A.1]{Marshall2011}. 
%     Since all steps held with iff we have shown the required result.
% \end{proof}

% \begin{proposition} \label{lem:simple-distortion-characterization}
%     Consider a vector $x \in \Re^n$ with $d$ distinct elements, which we store in $y \in \Re^d$. Let $c \in \N^d$ denote 
%     the number of copies of each component of $y$ in $x$. Then 
%     \begin{align*}
%         \bigcap_{\pi \in \Pi^n} \pi(x_{\uparrow} + \set{G}_n) &= \hull\left( \left\{\pi(x) \colon \pi \in \Pi^n\right\} \right) \\[-1em]   
%         &= \{ Sy \colon S\one_d = \one_n, \trans{\one}_n S = \trans{c}, S \geq 0\}.
%     \end{align*}
% \end{proposition}
% \begin{proof}
%     Let $\set{L}$ and $\set{M}$ denote the left and middle set respectively. We first show $\set{M} \subseteq \set{L}$. 
%     This follows from \cref{lem:permutation-hull-contained}, since $\set{M} \subset x_{\uparrow} + \set{G}_n$ and $\pi(\set{M}) = \set{M}$
%     for any $\pi \in \Pi^n$. For the reverse implication $\set{L} \subseteq \set{M}$ take some $v \in \set{L}$. 
%     Then by \cite[Cor.~2.B.3]{Marshall2011} we have $v \slt x$, which by \cref{lem:majorization} implies $v_{\uparrow} \in x_{\uparrow} + (\M^n)^\circ$. 
%     So by \cref{lem:permutation-hull-contained} we have $\pi(v) \in x_{\uparrow} + (\M^n)^\circ$ for all $\pi \in \Pi^n$. Applying $\pi^{-1} \in \Pi^n$ to both sides 
%     then implies $v \in \set{L}$. 
    
%     Since the doubly stochastic matrices are the convex hull of the permutation matrices \cite[2.A.2]{Marshall2011}, the convex hull of all permutations of $x$ iss
%     \begin{equation*}
%         \set{S} \dfn \left\{ H x \colon H \one_n = \one_n, \trans{\one}_n H = \one_n, H \geq 0 \right\}.
%     \end{equation*}
%     Consider
%     \begin{equation*}
%         \trans{C} \dfn \begin{bmatrix}
%             1 & \dots & 1 \\ &&& \ddots \\ &&&& 1 & \dots & 1
%         \end{bmatrix} \in \Re^{d \times n},
%     \end{equation*}
%     where row $i$ contains $c_i$ repetitions of $1$ for each $i \in [d]$ such that $x = C y$. The pseudo-inverse $C^{\dagger}$ is given as 
%     \begin{equation*}
%         C^{\dagger} \dfn \begin{bmatrix}
%             1/c_1 & \dots & 1/c_1 \\ &&& \ddots \\ &&&& 1/c_d & \dots & 1/c_d
%         \end{bmatrix} \in \Re^{d \times n}.
%     \end{equation*}
%     So $y = C^{\dagger} x$ and $C^{\dagger} C = I_d$. 

%     Take $H$ doubly stochastic. Then $v = H C C^{\dagger} x = HC y \in \set{S}$ and $S = HC$ satisfies the conditions above. 
%     Specifically  $H \trans{C} \one_d = H \one_n = \one_n$ and $\trans{\one_n} H \trans{C} = \trans{\one_n} \trans{C} = \trans{\one_d}$ and $H \trans{C} \geq 0$.
%     Let $\set{R}$ denote the right-most set in the statement of the lemma. We have shown $v \in \set{R}$ or $\set{R} \subseteq \set{S}$. 
%     For the reverse implication take some $v \in \set{R}$. So $v = S y = S C^{\dagger} C y = S C^{\dagger} x$. It is easy to verify that $S C^{\dagger}$ is doubly stochastic.
%     Thus $v \in \set{S}$. 
% \end{proof}

% \begin{proposition} \label{lem:inverse-cone-shift}
%     Consider some permutation invariant set $\set{A} \subseteq \Re^n$. Then 
%     \begin{equation*}
%         \set{A} = \bigcap_{\pi \in \Pi^n} \pi \left( \set{A} + (\M^n)^\circ \right). 
%     \end{equation*}
% \end{proposition}
% \begin{proof}
%     We first show $\cap_{\pi} \pi \left( \set{A} + (\M^n)^\circ \right) \subseteq \set{A}$. Assume $x \in \set{A}$. We have 
%     $\set{A} + (\M^n)^\circ = \{y + s \colon y \in \set{A}, s \in (\M^n)^\circ\} \supset \{y \colon y \in \set{A}\} = \set{A}$,
%     where the $\supset$ follows from $0 \in (\M^n)^\circ$. Hence $x \in \set{A} +(\M^n)^\circ$. We can make the same argument 
%     for any permutation $\pi(\set{A} + (\M^n)^\circ) \supset \pi(\set{A})$, since $\pi(\set{A}) = \set{A}$. Hence $x \in \cap_{\pi} \pi \left( \set{A} + (\M^n)^\circ \right)$. 

%     To show $\set{A} \subseteq \cap_{\pi} \pi \left( \set{A} + (\M^n)^\circ \right)$ we proceed by contradiction. Assume 
%     that there is some $x \in \set{A}$ such that $x \notin \cap_{\pi} \pi \left( \set{A} + (\M^n)^\circ \right)$. 
%     That is, there exists some permutation $\pi$ such that $x \notin \pi \left( \set{A} + (\M^n)^\circ \right)$. 
%     This holds iff $\pi^{-1}(x) \notin \set{A} + (\M^n)^\circ$. 

%     Since $\pi^{-1}$ is also a permutation there is thus some $\pi \in \Pi^n$ such that $\pi(x) \notin \set{A} + (\M^n)^\circ$. 
%     Note however that $x_{\uparrow}$ is also in $\set{A}$ by permutation invariance. Moreover by \cref{lem:permutation-hull-contained} $s = x - x_{\uparrow} \in (\M^n)^\circ$
%     for all $x \in \Re^n$. Hence $s = \pi(x) - x_{\uparrow} \in (\M^n)^\circ$ for all $\pi \in \Pi^n$. Thus there is some $s \in (\M^n)^\circ$ and some 
%     $y = x_{\uparrow} \in \set{A}$ such that $\pi(x) = x_{\uparrow} + s$. Therefore $\pi(x) \in \set{A} + (\M^n)^\circ$, which contradicts 
%     our initial assumption.
% \end{proof}

% \todo*{Can we show both previous statements simultaneously?}
% \begin{theorem} %\label{lem:inverse-cone-shift}
%     Consider some convex $\set{A} \subseteq \Re^n$. Then 
%     \begin{equation*}
%         \hull\left( \bigcup_{\pi \in \Pi^n} \pi(\set{A} \cap \M^n) \right) = \bigcap_{\pi \in \Pi^n} \pi \left( \set{A} + (\M^n)^\circ \right). 
%     \end{equation*}
% \end{theorem}
% \begin{proof}
%     Let $\set{L}$ and $\set{R}$ denote the left- and right-hand side set respectively. We first show $\set{L} \subseteq \set{R}$. 
%     Assume $x \in \set{L}$. That is, there are some $v^{(i)}_{\uparrow} \in \set{A}$ and $\pi^{(i)} \in \Pi^n$ for $i \in [m]$ such that 
%     $x \in \hull(\{\pi^{(i)}(v^{(i)}_{\uparrow})\}_{i=1}^m)$. By \cref{lem:permutation-hull-contained} we also have $\pi^{(i)}(v^{(i)}_{\uparrow}) \in \set{R}$
%     for all $i \in [m]$. Also note that, by convexity of $\set{A}$, $\set{R}$ is also convex. Hence any convex combination of $\{\pi^{(i)}(v^{(i)}_{\uparrow})\}_{i=1}^m$
%     should be in $\set{R}$, implying that $x$ is. 

%     Next we show that $\set{R} \subseteq \set{L}$. We proceed by contradiction, assuming $x \in \set{R}$ and $x \notin \set{L}$. 
%     Consider the set of vectors such that $x \in \hull(\{\pi(v) \colon \pi \in \Pi^n\})$,
%     which corresponds with $\{v \colon x \slt v\}$ by \cite[Cor.~2.B.3]{Marshall2011}. Take some $v$ in this set. 
%     Assume $v_{\uparrow} \in \set{A}$ then clearly $\hull(\{\pi(v) \colon \pi \in \Pi^n\}) \subseteq \set{L}$
%     so $x \in \set{L}$, which contradicts our assumption. So we have shown that for any $v \sgt x$ we have
%     $v_{\uparrow} \notin \set{A}$. \todo*{Stuck \dots}


% \end{proof}

% For the next part we will consider minimization of convex separable functions over $(\M^n)^\circ$. Specifically
% \begin{equation}
%     \min_{s \in (\M^n)^\circ} \quad \varphi(x + s) \dfn \sum_{i=1}^{n} \phi_i(x_i + s_i).
% \end{equation}
% We begin by formulating the problem in terms of the convex conjugate and the ordered conjugate from \cref{eq:ordered-conjugate}.

% \begin{lemma} \label{lem:infimum-dual-monotone}
%     For any convex function $\varphi \colon \Re^n \to \eRe$
%     \begin{equation} \label{eq:minimization-at-hand}
%         \inf_{s \in (\M^n)^\circ} \, \varphi(x + s) = (\varphi^*)^\diamond(x).
%     \end{equation}
% \end{lemma}
% \begin{proof}
%     Note that $s \in (\M^n)^\circ$ holds iff $\<\lambda, s\> \geq 0$ for all $\lambda \in \Re^n_{\uparrow}$ by definition of the 
%     dual cone. Alternatively $\sup_{\lambda \in \Re^n_{\uparrow}} -\<\lambda, s\>$ should be finite. This allows us to 
%     write a saddle problem associated with \cref{eq:minimization-at-hand}
%     \begin{equation*}
%         \inf_{s \in \Re^n} \, \sup_{\lambda \in \Re^n_{\uparrow}} \, \varphi(x+s) - \<s, \lambda\>. 
%     \end{equation*}
%     This, using strong duality\todo{cite!} and a change of variables with $y = x+s$, allows us to write the dual of \cref{eq:minimization-at-hand} 
%     \begin{align*}
%         &\sup_{\lambda \in \Re^n_{\uparrow}} \, \left( \inf_{s \in \ne_nRe^n} \, \varphi(y) - \<y, \lambda\> \right) + \<y, \lambda\>\\
%         &\sup_{\lambda \in \Re^n_{\uparrow}} \, - \left( \sup_{s \in \Re^n} \, \<y, \lambda\> - \varphi(y) \right) + \<x, \lambda\>.
%     \end{align*}
%     Plugging in the definition of the convex conjugate for the inner suprema and the ordered conjugate \cref{eq:ordered-conjugate} gives 
%     $(\varphi^*)^\diamond(x)$, completing the proof.
% \end{proof}
