# Supplementary material for: Ordered Risk Minimization: Learning More from Less Data
Source: arXiv:2303.09196 source file (2023-09-18)
Supplement: Supplementary file 4 [file statistics.tex]

\section{Statistical Framework} \label{app:statistical-framework}

\paragraph*{Proof of \cref{thm:distortion-bound}}
For continuous $Z$, \eqref{eq:distortion-bound} follows directly from \cref{eq:known-distortion-bound} and \cref{thm:elementary-coverage}. Conditioned on 
the event that the coverages $W$, as defined in \cref{thm:elementary-coverage} lie within $\distort$, the supremum upper bounds the right-hand side of 
\cref{eq:known-distortion-bound} and hence $\E[Z]$. As $W$ is uniformly distributed by \cref{thm:elementary-coverage} 
this event has probability $\prob[W \in \distort]$, confirming the stated result.

For discontinuous $Z$ the proof is more involved. Now \cref{thm:elementary-coverage} no longer holds, implying that $W$ defined 
there is not uniformly distributed over $\Delta^n$. Let $F(z) = \prob[Z \leq z]$ denote the cdf and $F(z-) = \prob[Z < z]$.
For the sample $\{Z_i\}_{i=1}^{n}$ let 
\begin{equation*}
    \tilde{F}_i = (1 - U_i) \cdot F(Z_i-) + U_i \cdot F(Z_i),
\end{equation*}
with the auxiliary random variables $U_i \deq \mathcal{U}(0, 1)$ for $i \in [n]$. Then $\tilde{F}_i \deq \mathcal{U}(0, 1)$ by \cite[Prop.~1.3]{Pflug2007}.
Therefore
\begin{equation*}
    \widetilde{W} = \left(\tilde{F}_{(i)} - \tilde{F}_{(i-1)} \right)_{i=1}^n.
\end{equation*}
is uniformly distributed over $\Delta^n$ (cf. \cite[\S6.4]{David2003}). We show that $\widetilde{W} \in \distort$ implies 
$W = (F(Z_{(i)}) - F(Z_{(i-1)}))_{i=1}^{n} \in \distort$ with probability one. Then the stated result follows from similar arguments as for the continuous case.

Since $\distort = \distort + (\M^n)^\circ$ and we assume $\widetilde{W} \in \distort$, we should show $W \in \widetilde{W} + (\M^n)^\circ$,
or equivalently $W - \widetilde{W} \in (\M^n)^\circ$. We assumed that $Z_{(n)} \geq \esssup[Z]$ and $Z_{(0)} = -\infty$. 
So $F(Z_{(n)}) = \tilde{F}_{(n)} = 1$ and $F(Z_{(0)}) = \tilde{F}_{(0)} = 0$. Thus $\sum_{i=1}^{n} W_i = \sum_{i=1}^{n} \widetilde{W}_i = 1$.
Therefore, by \cref{prop:dual-monotone-cone}, $W - \widetilde{W} \in (\M^n)^\circ$ holds iff, for all $k \in [n-1]$
\begin{align}
    & &\ssum_{i=1}^{k} W_i - \widetilde{W}_i &\geq 0 \nonumber \\
    &\Leftrightarrow &F(Z_{(k)}) - F(Z_{(0)}) - (\tilde{F}_{(k)} - \tilde{F}_{(0)}) &\geq 0 \nonumber \\
    &\Leftrightarrow &F(Z_{(k)}) - \tilde{F}_{(k)}&\geq 0. \label{eq:cdf-ineq-final}
\end{align}
The second $\Leftrightarrow$ follows from $F(Z_{(0)}) = \tilde{F}_{(0)} = 0$. W

Thus it is sufficient to show that \cref{eq:cdf-ineq-final} holds with probability one.
We proceed by contradiction, assuming that 
\begin{equation*}
    F(Z_{(k)}) < F(Z_{\pi(k)}) U_{\pi(k)} + F(Z_{\pi(k)} -) (1 - U_{\pi(k)}),
\end{equation*}
where $\pi$ be a permutation such that $\tilde{F}_{\pi(k)} = \tilde{F}_{(k)}$.
This holds only if $F(Z_{(k)}) < F(Z_{\pi(k)})$, which implies $F(Z_{(k)}) \leq F(Z_{\pi(k)}-)$. 
Thus, by monotonicity of $F$, $Z_{(k)} < Z_{\pi(k)}$. Let $\set{I} \dfn \{i \colon Z_i \leq Z_{(k)}\}$
or in words the indices associated with $Z_{(1)} \leq \dots \leq Z_{(k)} = Z_{(k+1)} = \dots = Z_{(k+\ell)}$,
where $\ell$ could be any nonnegative integer such that $k+\ell \leq n$. So by construction
$|\set{I}| \geq k$ and by monotonicity $\max_{i \in \set{I}} F(Z_i) = F(Z_{(k)})$. 
Therefore $F(Z_i) < F(Z_{\pi(k)})$ and $F(Z_i) \leq F(Z_{\pi(k)}-)$ for all $i \in \set{I}$.
We condition on the event $[U_i > 0, \, \forall i \in \set{I}]$, which has probability one.
Then $\tilde{F}_i < \tilde{F}_{(k)}$ for all $i \in \set{I}$. However, earlier we showed that
$|\set{I}| \geq k$. Thus $\tilde{F}_{(k)}$ cannot be the $k$'th largest element. So by contradiction 
we have shown that \cref{eq:cdf-ineq-final} holds with probability one. The earlier arguments then complete the proof. \qed
