# Supplementary material for: Ordered Risk Minimization: Learning More from Less Data
Source: arXiv:2303.09196 source file (2023-09-18)
Supplement: Supplementary file 5 [file tractable.tex]

\section{Tractable Reformulations} \label{app:conic-risk}
We review tractable reformulations of the proxy costs presented in this work. All of these are often referred to as \emph{risk measures} in literature \cite{Schuurmans2023}.
Specifically the ones we consider are \emph{conic-representable}, the consequences of which are discussed in this section.
We also highlight dedicated algorithms from literature, whenever they exist.
\subsection{Conic representable ambiguity}
We begin by considering the general class of conic representable risk measures \cite{Schuurmans2023}.
\begin{theorem} \label{thm:conic-ambiguity}
    For matrices $E \in \Re^{d \times n}$ and $F \in \Re^{d \times r}$ and some cone $\set{K}$. Let
    \begin{equation} \label{eq:conic-ambiguity-set}
        \amb = \left\{ \mu \in \Delta^n \colon \exists \nu \in \Re^r \colon E \mu + F \nu \leqc{\set{K}} b \right\},
    \end{equation}
    denote the ambiguity set with $\rho(X) = \sup_{\mu \in \amb} \<\mu, X\>$.
    If $\set{K}$ is polyhedral (i.e. it is represented by an intersection of halfplanes) or $\ri \amb \neq \emptyset$, then
    \begin{equation} \label{eq:dual-risk-representation}
        \begin{alignedat}{2}
            \rho(X) =& \min_{(\lambda, \tau)  \in \set{K}^* \times \Re} &\quad & \tau + \<b, \lambda\>\\
            &\sttshort&& \trans{E} \lambda + \tau \geq X, \, \trans{F} \lambda \geq 0.
        \end{alignedat}
    \end{equation}
\end{theorem}
\begin{proof}
    First note that \cref{eq:dual-risk-representation} is the Lagrangian dual associated with $\rho(X) = \sup_{\mu \in \amb} \<\mu, X\>$.
    Specifically, we can rewrite the supremum in standard dual form as
    \begin{equation*}
        \rho(X) = \left\{ \max_{y} \<(X, 0), y\> \colon  \begin{bmatrix} E & F \\ -\trans{\one_n} & 0 \\ \trans{\one_n} & 0 \end{bmatrix} y \leqc{\set{G}^*} \begin{bmatrix} b \\ 0 \\ 1 \end{bmatrix} \right\},
    \end{equation*}
    with $\set{G}^* = \set{K} \times \Re^n_+ \times \{0\}$ and $y = (\mu, \nu)$. Its dual is given as $\set{G} = \set{K}^* \times \Re^n_+ \times \Re$. 
    The primal is \cite[Ex.~5.12]{Boyd2004}
    \begin{equation}
        \begin{alignedat}{2}
            \rho(X) =& \min_{x \in \set{G}} &\quad & \<(b, 0, 1), x\>\\
            &\sttshort&& \begin{bmatrix} \trans{E} & - \one_n & \one_n \\ \trans{F} & 0 & 0 \end{bmatrix} = \begin{bmatrix} b \\ 0 \end{bmatrix}.
        \end{alignedat}
    \end{equation}
    If we partition $x = (\lambda, \beta, \tau)$ and eliminate $\beta$ from the above problem then \cref{eq:dual-risk-representation} is recovered. 
    The conditions on $\set{K}$ and $\ri \amb$ follow from the discussion at the start of \cite[\S{}5.2.3]{Boyd2004}.
\end{proof}

\begin{remark}
    Consider \cref{eq:robustified-erm} with $L(\theta) \colon \Re^{n_\theta} \to \Re^n$ convex.
    Then the dual problem for $\rho[L(\theta)]$ in \cref{eq:dual-risk-representation} has the constraint 
    \begin{equation*}
        \trans{E} \lambda + \tau \geq L(\theta),
    \end{equation*}
    which is clearly convex. The constraint can be made conic through application of an epigraph trick on $L(\theta)$. 
\end{remark}

Besides the classical positive orthant $\Re^n_+$, which is self dual, we will need two more cones below.
The exponential cone in $\Re^3$ and its dual are:
\begin{align*}
    \set{E}^3 &\dfn \{x \colon x_1 \leq x_2 \log(\tfrac{x_3}{x_2}), x_2 > 0\}, \, \\
    (\set{E}^3)^* &= \{y \colon y_1 < 0, y_3 > 0, -y_1 \log(\tfrac{-y_1}{y_3}) + y_1 - y_2 \leq 0\}.
\end{align*}
The second-order cone is self dual and is given as:
\begin{equation*}
    \set{Q}^n \dfn \{x = (t, z) \in \Re^{n+1} \colon  t \geq \nrm{y}_2\}.
\end{equation*}

\subsection{Distortion risk}
Optimizing distortion risks has been considered in literature before and dedicated algorithms were developed \cite{Mehta2022}. 
For purpose of generality we provide a reformulation in terms of \cref{thm:conic-ambiguity}.
\begin{proposition} \label{prop:distortion-ambiguity}
    Let $\rho$ be a distortion risk with $\distort \dfn \dom \rho^{\diamond} = \mu_{\uparrow} + (\M^n)^\circ$ 
    for some $\mu \in \Delta^n$. 
    Then the ambiguity set $\amb \dfn \dom \rho^*$ is given as:
    \begin{align*}
        \amb = \left\{ S \bar{\mu} \colon S \one_d = \one_n, \trans{\one}_n S = c, S \geq 0 \right\},
    \end{align*}
    with $\bar{\mu} \in \Re^d$ containing the $d \leq n$ unique elements of $\mu$ and $c \in \Re^d$ the number of copies of each element of $\bar{\mu}$ in $\mu$. 
    Moreover    
    \begin{equation} \label{eq:dual-distortion-representation}
        \begin{alignedat}{2}
            \rho(X) =& \min_{y, w} &\quad & \trans{\one_n}y + \trans{c} w \\
            &\sttshort&& y_i + w_j \geq X_i \bar{\mu}_j, \, (i, j) \in [n] \times [d].
        \end{alignedat}
    \end{equation}
\end{proposition}
\begin{proof}
    This follows from \cref{prop:fundamental-equivalence-lemma} and \cref{lem:simple-distortion-characterization}.
    For the final result, first note that $\amb$ can be written as in \cref{thm:conic-ambiguity} with constraints $I_n \mu - (\trans{\bar{\mu}} \kron I_n) \nu = 0$,
    $(\trans{\one_d} \kron I_n) \nu = \one_n$, $(I_d \kron \trans{\one_n})  = \one_d$ and $\nu = \vec(S) \geq 0$, with $\kron$ the Kronecker product and $\vec$ the vectorization operation. 
    Dualizing and simplifying gives the required result. Note that the associated cones are all polyhedral. Hence \cref{thm:conic-ambiguity} is applicable. 
\end{proof}

A similar characterization was provided in \cite[Thm.~4.3]{Bertsimas2009b}, which did not exploit sparsity of $\mu$ as we do. 
Note how for $\bar{\CVAR}$ we have $d = 4$ for any value of $n$. This fixed sparsity means that the number of constraints and variables in \cref{eq:dual-distortion-representation}
grow linearly with $n$. Without exploiting sparsity, the growth would be quadratic.

\subsection{$\phi$-divergences}
Optimization of $\phi$-divergence based risk measures has been considered in \cite{Ben-Tal2013} and \cite{Chouzenoux2019}.
Specifically \cite[Prop.~9]{Chouzenoux2019}:
\begin{equation*}
    \rho(X) = \min_{(\lambda, \mu) \in \Re_+ \times \Re} \, \lambda \alpha + \mu + \frac{1}{n} \sum_{i=1}^{n} \lambda \phi^* \left( \frac{X_i - \mu}{\lambda} \right).
\end{equation*}
This formulation is especially useful as it supports stochastic gradient descent algorithms \cite{Chouzenoux2019}. 

To support reformulating $\rho(X)$ as a conic program in the convex case, 
we also characterize the ambiguity sets associated with the $\phi$-divergences listed in \cref{tab:phi-table} in terms of conic constraints.
The associated risk measure can be minimized through application of \cref{thm:conic-ambiguity}. For all, except the Burg Entropy and $\chi^2$-distance 
we follow \cite[App.~A]{Schuurmans2023}.

\paragraph*{KL-divergence}
\begin{align*}
    &I_{\phi}(\mu, \one_n/n) \leq \alpha \, \Leftrightarrow \, \tfrac{1}{n} \ssum_{i=1}^{n} \log(n \mu_i) \leq \alpha \\
    &\Leftrightarrow \quad  \exists \nu \in \Re^n \colon \begin{cases}
        \log(\mu_i n) / n \leq \nu_i, \quad \forall i \in [n] \\
        \sum_{i=1}^{n} \nu_i \leq \alpha,
    \end{cases} \\
    &\Leftrightarrow \quad  \exists \nu \in \Re^n \colon \begin{cases}
        (-\nu_i, 1/n, \mu_i) \in \set{E}^3, \quad \forall i \in [n] \\
        \sum_{i=1}^{n} \nu_i \leq \alpha.
    \end{cases}
\end{align*}

\paragraph*{Burg Entropy}
\begin{align*}
    &I_{\phi}(\mu, \one_n/n) \leq \alpha \, \Leftrightarrow \, \tfrac{1}{n} \ssum_{i=1}^{n} (n \mu_i - \log(n \mu_i) - 1) \leq \alpha \\
    &\Leftrightarrow \quad - \tfrac{1}{n} \log(n \mu_i) \leq \alpha \\
    &\Leftrightarrow \quad  \exists \nu \in \Re^n \colon \begin{cases}
        - \log(\mu_i n) / n \leq \nu_i, \quad \forall i \in [n] \\
        \sum_{i=1}^{n} \nu_i \leq \alpha,
    \end{cases} \\
    &\Leftrightarrow \quad  \exists \nu \in \Re^n \colon \begin{cases}
        (-\nu_i, 1/n, \mu_i) \in \set{E}^3, \quad \forall i \in [n] \\
        \sum_{i=1}^{n} \nu_i \leq \alpha.
    \end{cases}
\end{align*}

\paragraph*{Hellinger Distance}
Using the fact that 
\begin{equation*}
    I_{\phi}(\mu, \one_n/n) = \ssum_{i=1}^{n} \left(\sqrt{\mu_i} - \sqrt{\tfrac{1}{n}}\right)^2 = 2 \left(1 - \ssum_{i=1}^{n} \sqrt{\tfrac{\mu_i}{n}}\right),
\end{equation*}
we have
\begin{align*}
    &I_{\phi}(\mu, \one_n/n) \leq \alpha \, \Leftrightarrow \, \ssum_{i=1}^{n} \sqrt{\mu_i/n} \geq 1 - \alpha/2 \\
    &\Leftrightarrow \quad  \exists \nu \in \Re^n \colon \begin{cases}
        1 - \alpha/2 \leq \ssum_{i=1}^{n} \sqrt{1/n} \nu_i, \quad \forall i \in [n] \\
        \nu_i^2 \leq \mu_i.
    \end{cases}
\end{align*}
The second constraint can be reformulated as 
\begin{align*}
    \nu_i^2 \leq \mu_i &\Leftrightarrow 4\nu_i^2 \leq (\mu_i + 1 + \mu_i - 1) (\mu_i + 1 - (\mu_i - 1)) \\
        &\Leftrightarrow 4\nu_i^2 \leq  (\mu_i + 1)^2 - (\mu_i - 1)^2 \\
        &\Leftrightarrow \nrm{(2 \nu_i, \mu_i - 1)}_2 \leq \mu_i + 1 \\
        &\Leftrightarrow (\mu_i + 1, 2\nu_i, \mu_i - 1) \in \set{Q}^2.
\end{align*}

\paragraph*{$\chi^2$ Distance}
Using the fact that 
\begin{equation*}
    I_{\phi}(\mu, \one_n/n) = \tfrac{1}{n} \ssum_{i=1}^{n} \tfrac{(n\mu_i - 1)^2}{n \mu_i} = \sum_{i=1}^{n} (\mu_i - \tfrac{1}{n})^2/\mu_i,
\end{equation*}
we can rewrite 
\begin{align*}
    &I_{\phi}(\mu, \one_n/n) \leq \alpha \,\Leftrightarrow \, \ssum_{i=1}^{n} (\mu_i^2 - 2 \tfrac{\mu_i}{n} + \tfrac{1}{n^2})/\mu_i \leq \alpha \\
    &\Leftrightarrow \quad \ssum_{i=1}^{n} \mu_i - \tfrac{2}{n} + \tfrac{1}{\mu_i n^2} \leq \alpha \\
    &\Leftrightarrow \quad \ssum_{i=1}^{n} \tfrac{1}{\mu_i n^2} \leq \alpha + 1 \\
    &\Leftrightarrow \quad  \exists \nu \in \Re^n \colon \begin{cases}
        \ssum_{i=1}^{n} \nu_i/n^2 \leq \alpha+1, \quad \forall i \in [n] \\
        1/\mu_i \leq \nu_i.
    \end{cases}
\end{align*}
The second constraint can be reformulated as 
\begin{align*}
    1/\mu_i \leq \nu_i &\Leftrightarrow 4 \leq (\mu_i + \nu_i + \mu_i - \nu_i) (\mu_i + \nu_i - (\mu_i - \nu_i)) \\
    &\Leftrightarrow 4 \leq (\mu_i + \nu_i)^2 - (\mu_i - \nu_i)^2 \\
    &\Leftrightarrow \nrm{(2, \mu_i - \nu_i)} \leq \mu_i + \nu_i \\
    &\Leftrightarrow (\mu_i + \nu_i, 2, \mu_i - \nu_i) \in \set{Q}^2.
\end{align*}

\paragraph*{Total variation}
\begin{align*}
    &I_{\phi}(\mu, \one_n/n) \leq \alpha \, \Leftrightarrow \, \nrm{\mu - \one_n/n}_1 \leq \alpha \\ 
    & \quad \Leftrightarrow \, \exists \nu \in \Re^n \colon \begin{cases}
        - \nu_i \leq \mu_i - 1/n \leq \nu_i, \, \forall i \in [n] \\
        \ssum_{i=1}^{n} \nu_i \leq \alpha.
    \end{cases}
\end{align*}
